# Supplementary material for: Per-Context Reverse Curricula for Sparse-Reward Reinforcement Learning
Source: arXiv:2607.26417 source file (2026-10-11)
Supplement: Supplementary file 1 [file supplementary_results.tex]

% Supplementary results for "SCOUT: Per-Context Reset Curricula for
% Sparse-Reward Reinforcement Learning" (compiles standalone).
% arXiv ancillary document, non-anonymous.
% Cross-references between the two documents are fixed text in both directions
% (the main paper's "Fig.~A1" and "the supplement"; this document's "Table 2 of
% the main paper") and must be updated by hand if either numbering changes.
% Build:  latexmk -pdf supplementary_results  (from paper/AAAI_arxiv/)
\documentclass[letterpaper,10pt]{article}
\usepackage[hmargin=1.2in,vmargin=1in]{geometry}
\usepackage{amsmath}
\usepackage{amsfonts}
\usepackage{amsthm}
% Unnumbered restatement of the main paper's Proposition 1 (proved here).
\newtheorem*{mainprop}{Proposition~1}
% Match the main paper's font stack (aaai2027.sty loads newtxtext/helvet/courier).
\usepackage{newtxtext}
\usepackage{newtxmath}
\usepackage[scaled=.92]{newtxtt}
\usepackage[hyphens]{url}
\usepackage{graphicx}
\usepackage{booktabs}
\usepackage{array}
\usepackage{microtype}
\usepackage{caption}
\captionsetup{font=small,labelfont=bf,skip=6pt}
\usepackage{xcolor}
\setlength{\intextsep}{8pt plus 2pt minus 2pt}
\setlength{\textfloatsep}{10pt plus 2pt minus 2pt}

\setlength{\emergencystretch}{1.5em}
\makeatletter
\renewcommand\section{\@startsection{section}{1}{\z@}{-2.2ex \@plus -.5ex \@minus -.2ex}{1.4ex \@plus .2ex}{\normalfont\Large\bfseries}}
\renewcommand\subsection{\@startsection{subsection}{2}{\z@}{-1.8ex \@plus -.4ex \@minus -.2ex}{0.9ex \@plus .2ex}{\normalfont\large\bfseries}}
\makeatother

% Lettered appendix sections (AAAI convention); A-prefixed floats/equations so
% cross-document references stay unambiguous against main-paper numbers.

\graphicspath{{figures/}}

% Campaign-5 revision markers ported as-is: revcolor is black, so \rev renders
% normally.
\definecolor{revcolor}{rgb}{0,0,0}
\newcommand{\rev}[1]{{\color{revcolor}#1}}
% Campaign-6 revision markers (within-group external-rule parity), accepted:
% revbcolor is black, so \revb renders normally. Set it back to {0.62,0.08,0.08}
% to re-highlight the campaign-6 pass.
\definecolor{revbcolor}{rgb}{0,0,0}
\newcommand{\revb}[1]{{\color{revbcolor}#1}}
% Campaign-7 revision markers (review.md pass), accepted: revccolor is black, so
% \revc renders normally. Set it back to {0.62,0.08,0.08} to re-highlight the
% campaign-7 pass.
\definecolor{revccolor}{rgb}{0,0,0}
\newcommand{\revc}[1]{{\color{revccolor}#1}}

% Clickable cross-references, visually silent. Load last (cleveref after hyperref).
\usepackage[hidelinks]{hyperref}
\usepackage[capitalize]{cleveref}
\crefformat{equation}{Eq.~#2#1#3}
\crefname{appendix}{Appendix}{Appendices}
\crefalias{section}{appendix}
\crefalias{subsection}{appendix}

\title{\vspace{-2.5em}\textbf{SCOUT: Per-Context Reset Curricula for Sparse-Reward Reinforcement Learning}\\[4pt]
{\Large Supplementary Results}}
\author{
    Siddharth Aphale\textsuperscript{\rm 1},\ Ayushman Singh\textsuperscript{\rm 2}\\[4pt]
    \textsuperscript{\rm 1}Stanford University \quad \textsuperscript{\rm 2}Sesame AI\\
    \texttt{saphale@stanford.edu}, \texttt{ayushman@sesame.com}
}
\date{}

\begin{document}
\maketitle
\vspace{-1.5em}

This appendix gives the experimental protocols, reproducibility details, scaffold-construction
procedures, proof of Proposition~1, supporting conflict results, and controller ablations.

%===============================================================================
\section{Experimental details, protocols, and reproducibility}
\label{app:exp-details}
\cref{tab:setup} lists the nine settings. \cref{tab:baselines} gives the selection rule for each
baseline.

\begin{table}[!htb]
  \centering
  \caption{\textbf{Experimental settings.} Six natural settings (top) test scaffold access; the
  \rev{three} pacing conflict settings (bottom) test allocation \rev{and its granularity}. HER
  applies only to the goal-conditioned SAC settings.}
  \label{tab:setup}
  \footnotesize
  \setlength{\tabcolsep}{4pt}%
  \begin{tabular}{@{}llccc@{}}
    \toprule
    Setting & Scaffold operator & Learner & Observation & Train / held-out \\
    \midrule
    PointMaze Medium & geodesic reset progress & SAC+HER & low-dim goal-cond. & 100 / 50 \\
    PointMaze Large & geodesic reset progress & SAC+HER & low-dim goal-cond. & 100 / 50 \\
    MiniGrid MultiRoom & route-based reset progress & PPO & CNN, partial & 200 / 100 \\
    MiniGrid DoorKey & stage-based reset progress & PPO & CNN, partial & 200 / 100 \\
    In-air FetchPickAndPlace & reverse-curriculum starts & SAC+HER & low-dim goal-cond. & 100 / 50 \\
    Meta-World PickPlace & reverse-curriculum starts & SAC+HER & low-dim goal-cond. & 100 / 50 \\
    \midrule
    PickAndPlace pacing conflict & reverse-curriculum starts & SAC+HER & low-dim goal-cond. & 100 / 50 \\
    Meta-World push $\times$ shelf-place conflict & reverse-curriculum starts & SAC+HER & low-dim goal-cond. & 200 / 100 \\
    \rev{PickAndPlace within-group conflict} & \rev{reverse-curriculum starts} & \rev{SAC+HER} & \rev{low-dim goal-cond.} & \rev{100 / 50} \\
    \bottomrule
  \end{tabular}
\end{table}

\begin{table}[!htb]
  \centering
  \caption{\textbf{Baseline scaffold-level selection rules.} Conditions share their setting's
  full training stack, differing only in reset-cell choice.}
  \label{tab:baselines}
  \footnotesize
  \setlength{\tabcolsep}{4pt}%
  \begin{tabular}{@{}>{\raggedright\arraybackslash}p{0.225\linewidth}>{\raggedright\arraybackslash}p{0.46\linewidth}>{\raggedright\arraybackslash}p{0.255\linewidth}@{}}
    \toprule
    Baseline & Selection mechanism & Constants \\
    \midrule
    Target-start training & every rollout at $\ell=0$ (no scaffold) & --- \\
    Fixed scaffold level$^{\dagger}$ & every rollout at one constant level & $\ell=2$ (``fixed mid'') \\
    Random scaffold sampling & $\ell \sim \mathrm{Unif}\{0,\dots,L\}$ per rollout, competence-independent & --- \\
    Global annealing & shared schedule $\ell(t) = \mathrm{round}\!\big(L\max(0,\,1 - t/T_{\mathrm{anneal}})\big)$ & $T_{\mathrm{anneal}}$: $2000$ constructed / $3000$ Meta-World \\
    Synchronized reverse curriculum & every context's start progress decays $0.9 \to 0$ linearly, identically & --- \\
    Asynchronous global mixture$^{\dagger}$ & time-varying categorical over levels; $\ell{=}0$ mass grows with aggregate-success EMA & rate $0.05$; mass $0.1 \to 0.7$; easy floor $0.2$ \\
    RFCL-style local frontier & SCOUT's frontier transition, uniform context sampling, antistall disabled & frozen SCOUT thresholds \\
    \rev{Group frontier$^{\dagger\ddagger}$} & \rev{SCOUT's frozen rule, one pooled frontier and statistics per oracle group} & \rev{frozen SCOUT hyperparameters} \\
    \rev{PLR cells$^{\dagger}$} & \rev{rank-prioritized teacher over all $(x,\ell)$ cells by per-cell mean $|\mathrm{TD}|$, staleness-mixed} & \rev{$\beta{=}0.5$, $\rho{=}0.1$, $\alpha{=}0.3$, SCOUT floor/cap} \\
    \rev{ALP cells$^{\dagger}$} & \rev{learning-progress teacher over all cells, score $|s - s_{\mathrm{slow}}|$} & \rev{SCOUT temperature, floor, cap} \\
    \rev{RFCL advance rule$^{\dagger}$} & \rev{advance iff $\geq 3$ of last $5$ rollouts succeed; no retreat or antistall} & \rev{struggling-context weight $w = (1-\hat s) + 0.1$} \\
    \rev{ACED-style advance$^{\dagger}$} & \rev{threshold-triggered advance only; no retreat or antistall} & \rev{SCOUT $\tau_{\mathrm{high}}$} \\
    \rev{Anneal + balanced replay$^{\dagger\ddagger}$} & \rev{global annealing; SAC minibatch draws fixed per-group quotas} & \rev{$\mathrm{minibatch}/G$ per group; empty group cedes its quota} \\
    \bottomrule
  \end{tabular}
  \par\smallskip
  {\footnotesize\raggedright $\dagger$: conflict settings only.\quad
  \rev{$\ddagger$: consumes oracle group labels.}\quad
  Balanced replay differs in the minibatch, not the reset choice.\par}
\end{table}

\paragraph{Scaffold operators.}\label{app:methods} We define a hand-built $G(x,\ell)$ for each
environment family. In PointMaze, the reset places the point partway along the geodesic path from
the context's start to its goal. Larger $\ell$ starts closer to the goal. MiniGrid MultiRoom
resets the agent along the route to the goal. DoorKey maps levels to task stages: carrying the
key, at the locked door with the key, past the opened door, and next to the goal. Level
$\ell{=}0$ is the original task. Manipulation uses reverse-curriculum starts. The object is
placed partway along a solved trajectory toward the goal. For in-air goals, the reset also
creates a grasped configuration. The levels move back toward the target start, which is
$\ell{=}0$.

\paragraph{Controller coefficients.}\label{app:hparams} \cref{tab:hparams} lists the frozen
controller constants, which we selected on conflict development seeds
(\cref{app:additional}).
Scaffold axes use five levels with fractions $\{0,0.25,0.5,0.75,0.9\}$ on the continuous
settings and $\{0,0.25,0.5,0.75,1.0\}$ on MiniGrid. All settings use sparse $0/\!-\!1$
rewards, with HER's future strategy on the goal-conditioned settings (\cref{tab:setup}).
Algorithm~1 of the main paper gives the full controller loop.

\paragraph{Controller-window semantics.} One \emph{controller window} (equivalently controller
step) is one training iteration. The controller samples active cells (Eq.~1 of the main paper),
collects rollouts, updates per-cell statistics, and runs one frontier-transition pass (Eq.~2 of
the main paper). It checks every context for eligibility in each window. A transition direction
must hold for two consecutive eligible windows before the frontier moves. Per-cell statistics
persist when a frontier leaves a cell and later returns. A cell that has never been visited starts
with no evidence, so it cannot transition until it has accumulated $15$ rollouts. To form the
sampling distribution, the controller applies the softmax, the exploration floor, and then the
per-cell cap. It redistributes excess probability proportionally and renormalizes.

\paragraph{Seeds and banks.} We use five seeds for the settings that reuse earlier development
banks: the two PointMazes and in-air FetchPickAndPlace. We use six seeds for MiniGrid MultiRoom,
DoorKey, Meta-World PickPlace, and the PickAndPlace conflict. A second six-seed block confirms the
PickAndPlace conflict. The primary Meta-World conflict protocol also uses six seeds, with smaller
blocks for the robustness checks (\cref{app:conflict-search}, \cref{tab:mw-robust}). The
trajectory-derived and \revc{policy-derived} experiments (\cref{tab:auto};
\revc{\cref{tab:self}}) use three seeds for the continuous settings and six for DoorKey. Other experiments state
their seed counts with their results. The code release will include the bank-construction seeds
and SHA-256 hashes.

\paragraph{Metrics.} The primary metric is area under the held-out target-start learning curve
within each task. AUC is comparable only within a task because episode length varies across
levels. We also report final held-out success and the number of seeds solved. Held-out success is
\emph{success-once}: an episode succeeds if the environment's success indicator is true at any
step, rather than only at termination. For the within-task AUC experiments
(\revb{Table~1} of the main paper; \cref{tab:auto}), we report medians to reduce the influence of
an occasional non-solving seed. Conflict tables report means of the per-seed worst-group minima
(\cref{tab:mw-conflict}), except that the main constructed-conflict results use medians.
Learning-curve figures show mean $\pm$ standard deviation.

\rev{\paragraph{Evaluation counts and inference convention.} Each evaluation point averages a
fixed episode budget over the held-out contexts at $\ell=0$: $100$ episodes on the constructed
\revb{and within-group} conflicts ($50$ contexts $\times 2$ \revb{each}), $200$ on the
Meta-World conflict ($100 \times 2$), $100$ on the PointMazes, and $50$ on the MiniGrid
settings. For paired conflict comparisons, the primary uncertainty estimate is a seed-bootstrap
$95\%$ confidence interval for the median paired difference in worst-group AUC. We use
$10{,}000$ resamples of the six paired seeds. We report exact two-sided sign tests descriptively
as wins out of six. With six paired seeds, the smallest attainable two-sided $p$-value is
$0.031$. The primary family contains \revb{$27$} such tests: SCOUT against every baseline on the
two conflicts and the within-group experiment. No individual sign test survives a
Holm--Bonferroni correction for a family of this size. We therefore base the main comparisons on
the bootstrap intervals. Screens and ablations are exploratory and reported per comparison.}

\paragraph{Compute.} All training runs are CPU-only by protocol (\texttt{device="cpu"} in
every training configuration). GPU execution changes the numerical environment and is not part
of the protocol. We ran experiments in three Linux environments: a $20$-core NVIDIA DGX Spark
(Grace aarch64, $121$~GiB unified memory), a single cloud H100 node whose GPU remains idle under
this protocol ($221$~GiB host RAM), and CPU nodes on a university SLURM cluster ($20$ cores and
$32$~GB per job). One $2400$-iteration Fetch conflict run takes about $40$ minutes on the
$20$-core machine and up to five hours on the cluster CPU nodes. Six to seven concurrent
$16$-worker runs use all $20$ cores. The software versions are Python $3.11$--$3.12$, PyTorch
$2.12.1$, Gymnasium $1.3.0$, Gymnasium-Robotics $1.4.2$, MuJoCo $3.10.0$, Meta-World $3.0.0$,
MiniGrid $3.1.0$, and NumPy $2.4$--$2.5$.

\begin{table}[!htb]
  \centering
  \caption{\textbf{Frozen controller constants} (shared across every setting and condition).}
  \label{tab:hparams}
  \small
  \begin{tabular}{@{}llc@{}}
    \toprule
    Component & Symbol & Value \\
    \midrule
    Sampling score weights (Eq.~1, main paper) & $\lambda_h$ / $\lambda_p$ / $\lambda_{\mathrm{stale}}$ & $1.0$ / $0.2$ / $0.1$ \\
    Softmax temperature & $\tau$ & $0.5$ \\
    Exploration floor / per-cell cap & $\epsilon$ / $q_{\max}$ & $0.1$ / $0.5$ \\
    Transition thresholds (Eq.~2, main paper) & $\tau_{\mathrm{low}}$ / $\tau_{\mathrm{high}}$ & $0.15$ / $0.8$ \\
    Evidence gate & $n_{\min}$ & $15$ rollouts \\
    Transition cooldown & --- & $3$ controller windows \\
    Antistall limit & $N_{\mathrm{stale}}$ & $4$ \\
    Success EMA & $\beta$ & $0.2$ \\
    \bottomrule
  \end{tabular}
\end{table}

\paragraph{Learner hyperparameters.} The policy learners are custom single-file
implementations adapted from CleanRL. We fixed their hyperparameters before running the test
seeds and use the same values for every condition within a setting (\cref{tab:learner}).
Training length, replay capacity, exploration constants, and worker count vary by setting and
episode horizon. The code release will include these values in the run configurations.

\begin{table}[!htb]
  \centering
  \caption{\textbf{Learner hyperparameters} (fixed a priori; shared by every condition within
  a setting).}
  \label{tab:learner}
  \small
  \begin{tabular}{@{}ll@{}}
    \toprule
    \multicolumn{2}{@{}l}{\emph{SAC / SAC+HER (PointMaze, Fetch, Meta-World)}} \\
    \midrule
    Networks & MLP $(256,256)$, ReLU; double-Q critic; tanh-Gaussian actor \\
    Optimizer / learning rate & Adam, $3\times10^{-4}$ (actor, critics, entropy) \\
    Discount / target-update rate & $0.99$ / $0.005$ \\
    Entropy temperature & auto-tuned; target $-\dim(\mathcal{A})$, initial $0.2$ \\
    Minibatch / warmup & $256$ / $1{,}000$ transitions \\
    Gradient steps per iteration & $16$ ($32$ on in-air FetchPickAndPlace) \\
    Replay capacity & $2\times10^5$--$6\times10^5$ (per setting) \\
    HER & future strategy, $k=4$ (goal-conditioned settings) \\
    Exploration & random-action prob.\ $0.3$, action noise $0.2$ \\
                & \quad($0.1$ / $0.1$ on the PointMazes) \\
    \midrule
    \multicolumn{2}{@{}l}{\emph{PPO (MiniGrid)}} \\
    \midrule
    Encoder & Conv $3{\to}16$ and $16{\to}32$ ($2{\times}2$), MLP $(128,128)$, Tanh \\
    Optimizer / learning rate & Adam, $2.5\times10^{-4}$ \\
    Discount / GAE $\lambda$ & $0.99$ / $0.95$ \\
    Clip / epochs / minibatch & $0.2$ / $4$ / $1{,}024$ \\
    Entropy / value coef.\ / grad.\ norm & $0.01$ / $0.5$ / $0.5$ \\
    Episodes per iteration & $16$ \\
    \midrule
    \multicolumn{2}{@{}l}{\emph{Contrastive RL (strong-learner comparison)}} \\
    \midrule
    Critic & InfoNCE over in-batch negatives, representation dim $64$ \\
    Regularizer & logsumexp penalty $0.1$ \\
    Positives / actor & HER-future achieved goals / SAC actor and entropy \\
    \bottomrule
  \end{tabular}
\end{table}

{\color{revcolor}
\subsection{Baseline protocols, tuning provenance, and external-rule component map}
\label{app:protocols}
\cref{tab:baselines} gives the selection mechanism and constants for every baseline. Contexts
are drawn uniformly unless stated otherwise.

\paragraph{Official RFCL protocol.} The official implementation (Tao et al.\ 2024) runs on
the PointMaze Large bank with one hundred state-only demonstrations, sparse reward, and the
shared held-out evaluation. Each of the three seeds runs for one million steps.
\cref{fig:rfcl-official} shows the held-out learning curves used in the main-paper comparison.

\begin{figure}[!htb]
  \centering
  \includegraphics{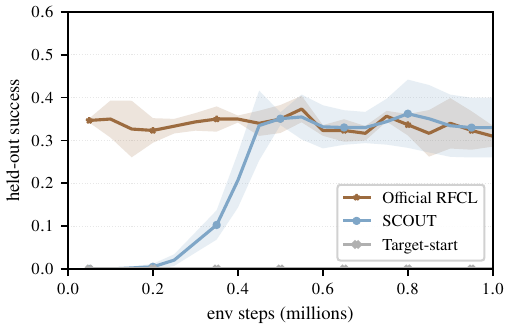}
  \caption{\textbf{Aligned official RFCL comparison on PointMaze Large} (held-out
  success-once, mean $\pm$ s.d., three seeds, shared $1$M-step budget). Official RFCL
  is near its plateau by the first checkpoint ($50$k steps), consistent with its
  ensemble critic and high update-to-data ratio; SCOUT reaches the same endpoint with
  plain SAC+HER and no demonstrations; target-start SAC+HER stays at zero.}
  \label{fig:rfcl-official}
\end{figure}

\paragraph{Tuning provenance.} Controller hyperparameters (score weights, thresholds,
$n_{\min}$, cooldown, hysteresis, antistall $N_{\mathrm{stale}}=4$, EMA $\beta=0.2$) were
selected on conflict development seeds (\cref{app:additional}) and frozen across every setting
and condition. ``Fixed mid'' was the best level on the development seeds. A full level sweep
confirms this choice (\cref{tab:fixed-sweep}): $\ell=2$ is the strongest constant on both
conflicts, and no constant exceeds $0.15$ worst-group final success on Meta-World. We also
screened the annealing length on development seeds (\cref{tab:anneal}). In a five-length screen
on the constructed conflict, no length solves the hard group; worst-group AUC is at most $0.017$
for every length. Thus, the default does not benefit from favorable selection. We set the
mixture coefficients before running the test seeds. The campaign conditions add no tuned
values. The group frontier inherits all fixed SCOUT hyperparameters, and the cell teachers use
the repository's existing PLR sampler defaults. We recorded every configuration before its runs
began. Evaluation seeds are 42--47. Development screens use 40--42, 42--44, or 50--52. We did
not select any configuration using final-test outcomes. \revb{The within-group runs of the four
external rules (\revc{Table~2} of the main paper) reuse these configurations on the unchanged
within-group bank. They add no tuned values and use evaluation seeds 42--47.}

\begin{table}[!htb]
  \centering
  \caption{\textbf{Fixed-level sweep} (both conflicts; worst-group AUC median / worst-group
  final median; levels 1--2 at six seeds where the block pre-exists, else three screen seeds).}
  \label{tab:fixed-sweep}
  \small
  \begin{tabular}{lcccc}
    \toprule
    Conflict & $\ell=1$ & $\ell=2$ (``fixed mid'') & $\ell=3$ & $\ell=4$ \\
    \midrule
    Constructed (wAUC / worst final) & 0.013 / 0.40 & \textbf{0.131} / \textbf{0.81} & 0.010 / 0.00 & 0.000 / 0.00 \\
    Meta-World (wAUC / worst final)  & 0.021 / 0.15 & \textbf{0.024} / 0.05 & 0.006 / 0.00 & 0.003 / 0.00 \\
    \bottomrule
  \end{tabular}
\end{table}

\begin{table}[!htb]
  \centering
  \caption{\textbf{Component map: SCOUT vs.\ the demonstration-anchored prior rules} as
  implemented in our component-matched baselines (main paper, Results). SCOUT's delta is the
  bidirectional transition (retreat $+$ antistall) and the general (non-demonstration) frontier
  index; the sampling scores are closely related.}
  \label{tab:component-map}
  \small
  \resizebox{\linewidth}{!}{%
  \begin{tabular}{@{}llll@{}}
    \toprule
    Component & SCOUT & RFCL (Tao et al.\ 2024) & ACED (Dai, Hofmann, and Williams 2021) \\
    \midrule
    Frontier index & task context $x$ & demonstration & demonstration section \\
    Assistance axis & ordered reset ladder (any semantics) & demo timestep & demo sections \\
    Advance & success EMA $\geq \tau_{\mathrm{high}}$, evidence $+$ cooldown & $\geq 3$ of last $5$ rollouts succeed & success threshold \\
    Retreat & success EMA $\leq \tau_{\mathrm{low}}$ & none & none \\
    Antistall & forced advance after $N_{\mathrm{stale}}$ idle windows & none & none \\
    Sampling & success-calibrated softmax, floor, cap & struggling-demo weighting & uniform over active sections \\
    Success statistic & EMA ($\beta = 0.2$), $n_{\min} = 15$ & rolling window ($5$) & running rate \\
    \bottomrule
  \end{tabular}}
\end{table}
}

%===============================================================================
\section{Scaffold construction: trajectory-derived and \revc{policy-derived}}
\label{app:auto}
The trajectory-derived extractor (main paper, Method) turns one successful reference trajectory
for each training context into a scaffold axis. It uses the same fixed progress quantiles across
tasks, except for the terminal DoorKey quantile, and a separate state codec for each environment.
We compare automatic and hand-built scaffolds using the retained gain ratio
\begin{equation}
R_{\mathrm{retain}} \;=\;
\frac{\mathrm{AUC}_{\mathrm{auto}}-\mathrm{AUC}_{\mathrm{true}}}
     {\mathrm{AUC}_{\mathrm{manual}}-\mathrm{AUC}_{\mathrm{true}}},
\label{eq:rretain}
\end{equation}
This ratio is the fraction of the hand-built scaffold's gain over target-start training that the
trajectory-derived scaffold recovers. A value at or above one means that the automatic scaffold
matches or exceeds the hand-built scaffold (\cref{tab:auto}).

\begin{table}[!htb]
  \centering
  \caption{\textbf{Trajectory-derived scaffolds retain the hand-built benefit.} \rev{Mean}
  held-out AUC \rev{on the block's common window}; $R_{\mathrm{retain}}\geq 1$
  (\cref{eq:rretain}) means the automatic scaffold matches or exceeds the hand-built one.
  \rev{CI: seed bootstrap of the mean-AUC ratio; DoorKey's is unstable, so point estimate
  only.} References differ from Table~1 of the main paper, whose DoorKey window closes before slow
  seeds solve.}
  \label{tab:auto}
  \small
  \resizebox{\linewidth}{!}{%
  \begin{tabular}{lcccccc}
    \toprule
    Setting & Target start & Manual SCOUT & Automatic SCOUT & $R_{\mathrm{retain}}$ & \rev{CI} & Invalid \\
    \midrule
    PointMaze Large & \rev{0.012} & \rev{0.225} & \rev{0.269} & \rev{1.21} & \rev{[1.05, 1.44]} & 0\% \\
    MiniGrid DoorKey & 0.259 & 0.451 & 0.541 & 1.47 & \rev{---} & 0\% \\
    In-air FetchPickAndPlace & \rev{0.002} & \rev{0.801} & \rev{0.845} & \rev{1.06} & \rev{[1.05, 1.06]} & 0\% \\
    \bottomrule
  \end{tabular}}
\end{table}

\paragraph{State codecs.} PointMaze stores the point position and velocity (the goal is fixed
by the context). DoorKey stores the encoded grid, agent pose, and any carried object.
FetchPickAndPlace stores the full MuJoCo state, including the actuator controls that hold a
grasp and the welded gripper mocap target. Without the actuator controls, a restored in-air
grasp opens and the object drops.

\paragraph{Offline validation.} Before RL begins, we restore every extracted state and run a few
settling steps. We check for finite observations, in-bounds object positions, and, for Fetch,
stable grasps. All three settings have a $0\%$ invalid-reset rate.

\paragraph{Reference trajectory sources.} PointMaze trajectories come from a shortest-path
planner. DoorKey trajectories come from a breadth-first solver that steps the environment. The
solver omits the final goal-reaching step, so the most assisted level is adjacent to the goal.
Fetch trajectories come from a four-phase scripted pick-and-place controller. Each source solves
every training context. \revc{On DoorKey, the fixed progress quantiles recover the key, door,
and goal progression without event labels.}

\subsection{\revc{Policy-derived scaffolds with fallback support}}
\label{app:self}
\rev{These experiments study post-training scaffold \emph{recycling and refinement}. The policy
that supplies the reference trajectories was first trained with a scaffold. The results show
that the scaffold axis can be derived again from the policy's own competence. They do not show
that scaffolds can be discovered from the unassisted sparse-reward problem.}
The trajectory-derived extractor does not depend on the source of the reference trajectory. We
test trajectories from the policy's \emph{own} first target-start success in each context. After
a scaffolded training run, we roll out the trained policy from each training context's target
start. We make $k{=}5$ stochastic attempts and retain the shortest successful trajectory. We
then pass its states through the same extractor and use the same controller. Every
\revc{policy-derived} ladder passes offline restore validation, with a $0\%$ invalid-reset
rate. The target-start and
manual baselines are the same runs used in the trajectory-derived comparison, with the window
matched to \cref{tab:auto}. Within this block, $R_{\mathrm{self}}$ compares the
\revc{policy-derived} and manual scaffolds.

We report a \emph{bootstrap fraction}, the share of contexts whose ladder is not a purely
unassisted self solution (bootstrapped by the scaffold-trained policy or, failing that, a
scripted fallback). This fraction indicates how much each ladder depends on prior scaffolding.

\begin{table}[!htb]\color{revccolor}
  \centering
  \caption{\textbf{Policy-derived scaffolds (with fallback support) retain the hand-built
  benefit.} Bootstrap fraction $=$ (bootstrapped $+$ scripted fallback)$/n_{\text{train}}$,
  lower more purely policy-derived; $R_{\mathrm{self}}\!\geq\!1$ matches the hand-built
  scaffold.}
  \label{tab:self}
  \small
  \begin{tabular}{lcccc}
    \toprule
    Setting & Bootstrap frac. & $R_{\mathrm{self}}$ & $>$ target (seeds) & Invalid \\
    \midrule
    MiniGrid DoorKey         & 0.005 & 1.76 & 5/6 & 0\% \\
    PointMaze Large          & 0.810 & 1.22 & 3/3 & 0\% \\
    In-air FetchPickAndPlace & 0.990 & 1.03 & 3/3 & 0\% \\
    \bottomrule
  \end{tabular}
\end{table}

\revc{\cref{tab:self} shows that policy-derived scaffolds retain the hand-built benefit in
all three settings. DoorKey is nearly fully policy-derived, with $0.5\%$ fallback, and slightly
exceeds the scripted trajectory-derived ladder ($R_{\mathrm{self}}=1.76$ vs
$R_{\mathrm{retain}}=1.47$).} For Fetch, $99\%$ of the trajectories come from the
scaffold-trained policy and none use the scripted fallback. PointMaze Large requires more
support. The policy solves only about one third of the contexts, so $65\%$ use the scripted
reference. As a result, $R_{\mathrm{self}}$ largely measures those fallback cells.

%===============================================================================
\section{Pacing conflicts: supporting results and the Meta-World conflict}
\label{app:conflicts}
This section gives the toy construction and proof behind Proposition~1, supporting analyses of
the constructed conflict, and results for the Meta-World conflict.

\subsection{The toy construction and proof of Proposition~1}
\label{app:toy}

The main paper states Proposition~1 with a one-sentence sketch. Here we give the full
construction and proof. The construction represents the scheduling conflict tested in the
experiments, rather than the full reinforcement learning dynamics.

Consider two contexts, $a$ and $b$, and two scaffold levels, $\ell=1$ (assisted) and $\ell=0$
(the target start). Each context receives the same budget $H=K+1$ training episodes, $K>1$.
Let $n_1(x)$ and $n_0(x)$ denote the number of assisted and target-start episodes assigned to
context $x$. Assume context $a$ succeeds at evaluation iff $n_1(a)\ge 1$ and $n_0(a)\ge K$,
and context $b$ iff $n_1(b)\ge K$ and $n_0(b)\ge 1$. Since $n_0(x)=K+1-n_1(x)$, these reduce to
\[
    a \text{ succeeds iff } n_1(a)=1, \qquad b \text{ succeeds iff } n_1(b)=K .
\]
Context $a$ needs assistance removed quickly; context $b$ needs it retained.

\begin{mainprop}[synchronized global pacing can be insufficient; restated]
For every $K>1$, there exists a two-context, two-level scaffold curriculum with per-context budget $K+1$
such that a context-local schedule solves both contexts, while every synchronized global schedule fails at
least one context.
\end{mainprop}

\begin{proof}
A synchronized global schedule gives both contexts the same assisted count $n_1$; context $a$
requires $n_1=1$ and context $b$ requires $n_1=K>1$, so every synchronized schedule fails at
least one context. A context-local schedule assigns $n_1(a)=1$ and $n_1(b)=K$, satisfying both
under the same per-context budget.
\end{proof}

\paragraph{Scope.} The construction rules out synchronized global schedules, not richer
population-level curricula that keep several levels available at once. For this reason, the main
paper includes an asynchronous global mixture. The construction compares the schedules they can
represent; it is not an optimality proof for SCOUT.

\subsection{Supporting results on the constructed conflict}
\label{app:extra}

\rev{\paragraph{Constructed conflict: granularity and external-rule comparison.}
\cref{tab:pnp_c5} reports the additional conditions on the constructed conflict. We compute all
values over the replication block's common window and pair each condition with that block's
SCOUT runs. The two blocks with the same protocol have medians of $0.354$ (main paper, Results)
and $0.378$. Their difference is $0.024$. The observed group-frontier difference is
$7.5\times$ this between-block variation.}

\begin{table}[!htb]\color{revcolor}
  \centering
  \caption{\textbf{Constructed conflict: added conditions} (six seeds; median worst-group AUC,
  mean $\pm$ s.d.\ worst-group final, paired median $\Delta$ (SCOUT $-$ condition);
  replication-block window). $\ddagger$: consumes oracle group labels. All conditions are
  specified in \cref{app:protocols}.}
  \label{tab:pnp_c5}
  \small
  \begin{tabular}{lcccc}
    \toprule
    Condition & Worst AUC & Worst final & $\Delta$ [CI] & SCOUT wins \\
    \midrule
    SCOUT & \textbf{0.378} & $0.97 \pm 0.04$ & (ref.) & --- \\
    Group frontier (oracle)$^{\ddagger}$ & 0.229 & $0.95 \pm 0.02$ & $+0.18\;[0.04, 0.29]$ & 5/6 ($p=0.22$) \\
    RFCL advance rule (no retreat) & 0.297 & $\mathbf{0.98 \pm 0.03}$ & $+0.13\;[-0.09, 0.30]$ & 4/6 ($p=0.69$) \\
    ACED-style advance (no retreat) & 0.083 & $0.60 \pm 0.24$ & $+0.30\;[0.23, 0.40]$ & 6/6 ($p=0.031$) \\
    PLR cells & 0.239 & $0.63 \pm 0.37$ & $+0.15\;[0.05, 0.35]$ & 6/6 ($p=0.031$) \\
    ALP cells & 0.123 & $0.81 \pm 0.36$ & $+0.25\;[0.13, 0.40]$ & 6/6 ($p=0.031$) \\
    \bottomrule
  \end{tabular}
\end{table}

\rev{\paragraph{Within-group frontier dispersion.} \cref{fig:c5variance} shows the mechanism
behind the granularity result (main paper, Results). It plots the per-window IQR of SCOUT's
frontiers within each oracle group. By the middle of training, the easy groups use a single
shared level. The hard groups retain one to two levels of dispersion on the constructed conflict
and up to four on shelf-place. At any time, more than half of the hard-group contexts differ from
their group's median level. A single pooled level cannot represent this variation.}

\begin{figure}[!htb]
  \centering
  \includegraphics[width=\linewidth]{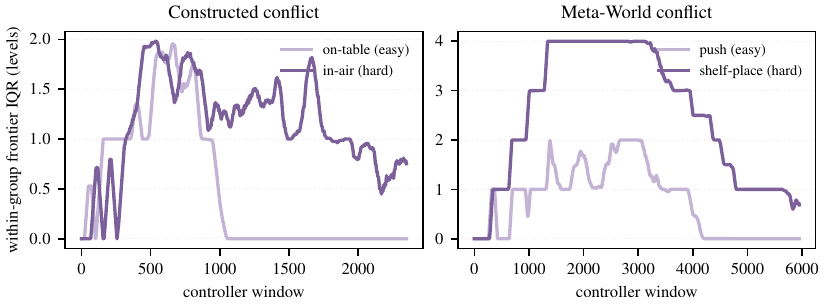}
  \caption{\rev{\textbf{Within-group frontier dispersion} (median over six seeds, smoothed;
  light $=$ easy group, dark $=$ hard group). SCOUT's per-context frontiers disperse
  substantially inside each oracle group, most strongly in the hard groups.}}
  \label{fig:c5variance}
\end{figure}

\rev{\paragraph{What aggregate metrics hide.} \cref{fig:c5masking} compares aggregate and
worst-group AUC. On the Meta-World conflict, aggregate held-out AUC varies by $1.2\times$ across
conditions, while worst-group AUC varies by ${\sim}50\times$. The three methods that fail on one
group are therefore within ${\sim}5\%$ aggregate AUC of the methods that maintain performance
on both groups. With equal group sizes, aggregate final success preserves the ranking. Our
masking claim therefore applies to aggregate AUC, not final success.}

\begin{figure}[!htb]
  \centering
  \includegraphics[width=\linewidth]{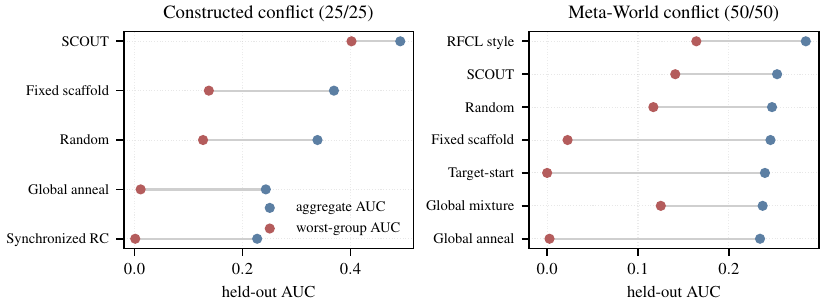}
  \caption{\rev{\textbf{Aggregate AUC vs.\ worst-group AUC per condition} (group sizes in
  titles). Failure on one group has little effect on aggregate AUC but sharply reduces
  worst-group AUC.}}
  \label{fig:c5masking}
\end{figure}

\subsection{A second pacing conflict on unmodified Meta-World tasks}
\label{app:conflict-search}
We screened natural context splits in MiniGrid DoorKey and Meta-World at reduced budgets, using
two to six seeds. None shows the two-sided opposition of the constructed conflict. We find one
consistent \emph{one-sided} conflict and evaluate it at the full protocol below. It pairs push
with shelf-place. Shelf-place does not learn from the target start but can learn from grasped
starts, while push tolerates assistance.

\paragraph{The push $\times$ shelf-place conflict.} We combine the two unmodified tasks in one
bank ($100$ train $+$ $50$ held-out contexts per task) under the same scaffold operator,
SAC+HER learner, and frozen controller as elsewhere, for $6000$ iterations over six seeds
(groups $=$ tasks). \cref{tab:mw-conflict} lists every condition. \rev{The main paper discusses
the campaign rows: the group frontier, advance-only rules, cell teachers, and balanced-replay
control. \cref{app:protocols} specifies their protocols.} The result also replicates on a second
software stack. SCOUT's frontiers follow the same pattern as in the constructed conflict. Push
reaches the target start early, while shelf-place retains assistance for most of training
(\cref{fig:mw_conflict}, panel 3).

\begin{figure}[!htb]
  \centering
  \includegraphics[width=\linewidth]{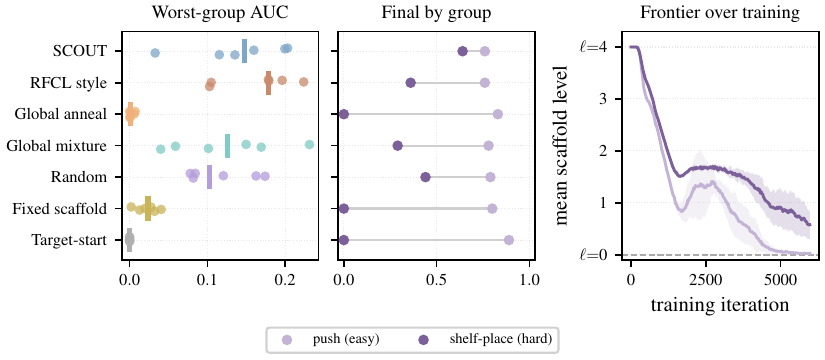}
  \caption{\textbf{The Meta-World conflict, in the format of Fig.~3 of the main paper.}
  \textbf{1:} worst-group AUC. \textbf{2:} final success by group; deterministic schedules
  fail on shelf-place. \textbf{3:} mean scaffold level by group: push advances early,
  shelf-place retains assistance far longer.}
  \label{fig:mw_conflict}
\end{figure}

\begin{table}[!htb]
  \centering
  \caption{\textbf{Meta-World push $\times$ shelf-place conflict} (six seeds, $6000$
  iterations, five-level scaffold; cells are seed means; best per column bold). Worst group
  $=$ within-seed minimum over the two tasks (iteration-axis AUC); ``SCOUT wins'' counts
  paired worst-group AUC wins (sign test, descriptive). \rev{$\ddagger$: consumes oracle task
  labels. The RFCL-style frontier keeps retreat; the RFCL advance rule is advance-only
  (\cref{app:protocols}).}}
  \label{tab:mw-conflict}
  \small
  \begin{tabular}{lccccc}
    \toprule
    Condition & Worst AUC & Push final & Shelf final & Worst final & SCOUT wins \\
    \midrule
    SCOUT                    & 0.141 & 0.743 & 0.617 & 0.613 & (ref.) \\
    \rev{Group frontier (oracle)$^{\ddagger}$} & \rev{\textbf{0.256}} & \rev{0.840} & \rev{\textbf{0.757}} & \rev{\textbf{0.720}} & \rev{0/6 ($p=0.031$)} \\
    RFCL-style local frontier & 0.164 & 0.743 & 0.373 & 0.367 & 3/6 ($p=1.0$) \\
    \rev{RFCL advance rule (no retreat)} & \rev{0.042} & \rev{0.763} & \rev{0.167} & \rev{0.123} & \rev{5/6 ($p=0.22$)} \\
    \rev{ACED-style advance (no retreat)} & \rev{0.049} & \rev{0.777} & \rev{0.313} & \rev{0.313} & \rev{6/6 ($p=0.031$)} \\
    \rev{PLR cells} & \rev{0.118} & \rev{0.683} & \rev{0.197} & \rev{0.197} & \rev{5/6 ($p=0.22$)} \\
    \rev{ALP cells} & \rev{0.140} & \rev{0.823} & \rev{0.477} & \rev{0.477} & \rev{3/6 ($p=1.0$)} \\
    Global annealing         & 0.003 & 0.843 & 0.000 & 0.000 & 6/6 ($p=0.031$) \\
    \rev{Anneal + balanced replay$^{\ddagger}$} & \rev{0.006} & \rev{0.803} & \rev{0.000} & \rev{0.000} & \rev{6/6 ($p=0.031$)} \\
    Asynchronous global mixture & 0.125 & 0.757 & 0.383 & 0.383 & 3/6 ($p=1.0$) \\
    Random scaffold          & 0.117 & 0.803 & 0.477 & 0.477 & 4/6 ($p=0.69$) \\
    Fixed mid scaffold       & 0.022 & 0.753 & 0.053 & 0.053 & 5/6 ($p=0.22$) \\
    Target start             & 0.000 & \textbf{0.880} & 0.000 & 0.000 & 6/6 ($p=0.031$) \\
    \bottomrule
  \end{tabular}
\end{table}

\paragraph{Horizon and ladder-resolution robustness.} Two follow-up blocks bound the result
(\cref{tab:mw-robust}). First, we increase the horizon to $9000$ iterations while keeping the
five-level protocol. Global annealing still ends at $0.000$ shelf-place success on all three
seeds. The failure therefore persists with more training. SCOUT reaches $0.680$, while the
mixture improves later and reaches $0.853$. Second, we use a nine-level ladder at the same
horizon. All methods then solve both tasks. A deterministic global schedule fails when the
ladder is too coarse for one pace to serve both groups. SCOUT solves shelf-place with either
ladder.

\begin{table}[!htb]
  \centering
  \caption{\textbf{Horizon and ladder-resolution robustness} of the push $\times$ shelf-place conflict
  (cells: worst-group AUC / shelf-place final). Annealing continues to fail with a longer horizon
  at five levels, but succeeds with nine levels.}
  \label{tab:mw-robust}
  \small
  \begin{tabular}{lccc}
    \toprule
    Protocol (ladder, budget, seeds) & SCOUT & Global annealing & Global mixture \\
    \midrule
    5 levels, 6000 it, 6 seeds & 0.141 / 0.617 & 0.003 / 0.000 & 0.125 / 0.383 \\
    5 levels, 9000 it, 3 seeds & 0.337 / 0.680 & 0.008 / 0.000 & 0.347 / 0.853 \\
    9 levels, 9000 it, 2 seeds & 0.367 / 0.840 & 0.353 / 0.890 & 0.374 / 0.810 \\
    \bottomrule
  \end{tabular}
\end{table}

\paragraph{Long-horizon level count.} A long-horizon DoorKey-16$\times$16 study (automatic
SCOUT, three seeds; ${\approx}2.3{\times}$ the 8$\times$8 horizon) tests the same issue for
scaffold access. Increasing the ladder from five to nine levels raises final success by
${\approx}0.10$ without reducing AUC. Thirteen levels provide little further benefit and reduce
AUC because the fixed budget spends too long at each level. Longer horizons can benefit from
more levels, but too many levels slow progression.

\paragraph{DoorKey pacing splits.} We also split DoorKey-8$\times$8 by geometry into short and
long solutions. We train each group at a single fixed scaffold level. No fixed level solves both
groups. The easy group remains at zero for every level and seed. The hard group reaches $0.74$
at only one intermediate level. In contrast, the same controller used as a curriculum solves
both groups, with final success of $1.00$ on the easy group and $0.92$ on the hard group. The
benefit comes from moving across levels rather than selecting one level. Constructed
DoorKey-16$\times$16 solution-length splits identify a boundary for the mixture baseline. SCOUT
outperforms global annealing on the worst group on all three seeds in two bank compositions,
with about $2\times$ the worst-group AUC. However, the asynchronous mixture ties SCOUT. This
result is consistent with cross-level transfer. MiniGrid restore states lie on the solution path
of the target-start task, and the convolutional policy generalizes across levels. Population-level
mixed exposure can therefore train $\ell{=}0$ directly.

\paragraph{Scope.} Together with the contrastive learner result (main paper, Results), the
DoorKey splits identify two cases in which SCOUT provides less benefit. A strong directed
learner can remove the \emph{access} problem, and strong cross-level generalization can substitute
for \emph{allocation}. The conflict setting instead requires chain-dependent tasks with weak
cross-level transfer.

%===============================================================================
\section{Ablations}
\label{app:additional}

\paragraph{Hyperparameter screens.} \cref{tab:antistall,tab:anneal} report the
development-seed screens behind the frozen controller constants (selection and freezing
protocol in \cref{app:protocols}). In the antistall screen, every enabled stale limit beats
the disabled controller on worst-group AUC and raises the hard group's final success to at least
$0.92$. Thus, antistall helps on these development seeds. Differences among
$N_{\mathrm{stale}}\in\{2,4,8\}$ are not monotonic and are small relative to the variation
across three seeds. The annealing length has little effect on PointMaze Large. Every tested
length gives a similarly low development-seed AUC.

\begin{table}[!htb]
  \centering
  \caption{\textbf{Antistall sweep} (conflict, three development seeds). Worst-group AUC is the
  median over seeds; final success columns are medians by group.}
  \label{tab:antistall}
  \small
  \begin{tabular}{lccc}
    \toprule
    $N_{\mathrm{stale}}$ & worst-group AUC & on-table final & hard final \\
    \midrule
    0 (off) & 0.15 & 0.96 & 0.84 \\
    2       & 0.49 & 1.00 & 1.00 \\
    4       & 0.20 & 1.00 & 0.92 \\
    8       & 0.39 & 1.00 & 0.96 \\
    \bottomrule
  \end{tabular}
\end{table}

\begin{table}[!htb]
  \centering
  \caption{\textbf{PointMaze Large annealing-length screen} (development seeds 40--42). Median
  held-out AUC and final success by schedule length $T_{\mathrm{anneal}}$.}
  \label{tab:anneal}
  \small
  \begin{tabular}{lcc}
    \toprule
    $T_{\mathrm{anneal}}$ & AUC & final \\
    \midrule
    1000 & 0.00 & 0.00 \\
    1500 & 0.05 & 0.00 \\
    2500 & 0.04 & 0.00 \\
    3500 & 0.03 & 0.00 \\
    5000 & 0.05 & 0.03 \\
    \bottomrule
  \end{tabular}
\end{table}

\paragraph{Critic uncertainty ablation.} Adding a critic uncertainty term to the sampling or
transition signal did not consistently improve performance. It could also delay progression
near sparse-reward discontinuities, so we exclude it. The code release will include full
per-seed tables and the conflict confirmation block.

\paragraph{Evidence-gated transition rules.} To test whether the EMA-threshold transition is
one possible stable local controller, we test two evidence-gated variants. They differ from
SCOUT only in the transition rule. \emph{TP-SCOUT} uses Wilson bounds over discounted success
counts, while \emph{B-SCOUT} uses a discounted Beta posterior. \cref{fig:rules} shows a six-seed
replication on the automatic conflict. All stable local-frontier rules perform similarly and
outperform both global schedules. Evidence gating reduces frontier reversals by about half at
the same worst-group AUC. On the coarser hand-built ladder, the gated rules perform somewhat
better. The success statistics must discount old evidence. An undiscounted posterior
($\gamma{=}1$) reduces worst-group AUC to $0.58$ because it cannot adapt to a changing policy.
We also tested a drift-aware Bayesian gate across $23$ tuned configurations. Its best
configuration uses no anticipation and still performs worse than every simple rule. These
results do not distinguish among the stable local rules. They indicate that the shared local
frontier, rather than one specific transition rule, provides the main benefit (main paper,
Results).

\begin{figure}[!htb]
  \centering
  \includegraphics[width=\linewidth]{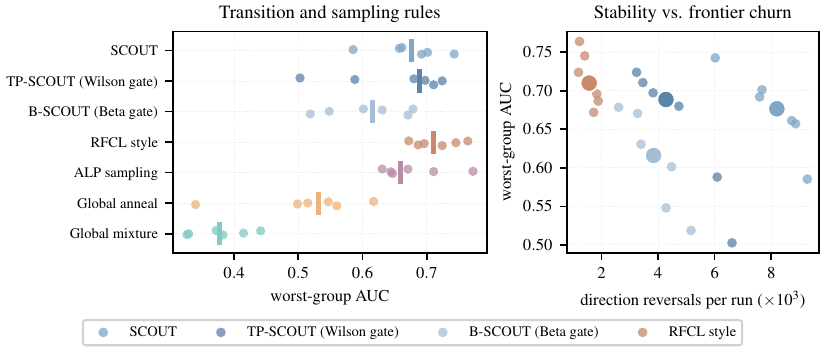}
  \caption{\textbf{Transition and sampling rules on the automatic constructed conflict} (six
  seeds; this block's common window). \textbf{Left:} worst-group AUC per rule (per-seed dots,
  median ticks): the stable local-frontier rules outperform both global schedules, with no
  significant pairwise differences among them. \textbf{Right:} per-context direction
  reversals against worst-group AUC (large markers medians): evidence gating halves reversals at
  equal worst-group AUC; the advance-biased RFCL-style rule churns least.}
  \label{fig:rules}
\end{figure}

\end{document}
